# Supplementary material for: From Counting Stations to City-Wide Estimates: Data-Driven Bicycle Volume Extrapolation
Source: arXiv:2406.18454 source file (2024-08-01)
Supplement: Supplementary file 1 [file Flowchart_data_cleaning.tex]

\subsection{Flow chart data cleaning bike-sharing data}
% include a flow chart here! https://www.overleaf.com/learn/latex/LaTeX_Graphics_using_TikZ%3A_A_Tutorial_for_Beginners_(Part_3)%E2%80%94Creating_Flowcharts
%define shape of box
\tikzstyle{box} = [rectangle, rounded corners, minimum width=3cm, minimum height=0.7cm,text centered, draw=black]
% define shape of arrows
\begin{center}
\begin{figure}

\tikzstyle{arrow} = [thick,->,>=stealth]
%Set up the environment for flow chart
    % Define the boxes
\begin{tikzpicture}[node distance=1.5cm]
\node (start) [box, yshift=0.1cm] {Original Number of trips (2,086,484)};
\node (in2) [box, below of=start, yshift=0.3cm] {Remove trips between 20-100m (n=13,385)};
\node (in3) [box, below of=in2, yshift=0.3cm] {Remove trips longer than 45km (n=100)};
\node (in4) [box, below of=in3, yshift=0.3cm] {Remove trips shorter than 90sec (n=34,107)};
\node (in5) [box, below of=in4, yshift=0.3cm] {Remove trips longer than 10h (n=126,161)};
\node (in6) [box, below of=in5, yshift=0.3cm, xshift=-4cm] {Remove trips slower than 2km/h  (n=345,828)};
\node (in7) [box, below of=in5, yshift=0.3cm, xshift=4cm] {Remove trips faster than 40km/h (n=226,842)};
\node (end) [box, below of=in6, yshift=0.5cm, xshift=4cm] {Number of trips remaining (1,339,737)};
    % Define the arrows
\draw [arrow] (start) -- (in2);
\draw [arrow] (in2) -- (in3);
\draw [arrow] (in3) -- (in4);
\draw [arrow] (in4) -- (in5);
\draw [arrow] (in4) -- (in5);
\draw [arrow] (in5) -- (in6);
\draw [arrow] (in5) -- (in7);
\draw [arrow] (in6) -- (end);
\draw [arrow] (in7) -- (end);
\end{tikzpicture}
\caption{The cleaning of the bike sharing data with the various steps taken.}
\label{fig:flowchart_cleaning_bikesharingdata}
\end{figure}
\end{center}
