# Supplementary material for: From Counting Stations to City-Wide Estimates: Data-Driven Bicycle Volume Extrapolation
Source: arXiv:2406.18454 source file (2024-08-01)
Supplement: Supplementary file 2 [file feature_importance_MAE.tex]

\begin{figure}[H]
  \begin{subfigure}{7cm}
    \centering
    \includegraphics[width=\textwidth]{Graphs/feature_importance_dailyMAE.png}
    \caption{Daily level}
    \label{figure:feature_importance_daily_MAE}
  \end{subfigure}
\caption{Information gain computed via a grouped version of permutation importance for both the XGBoost model at the daily level using MAE.}
\label{fig:feature_importance}
\end{figure}
